# Supplementary material for: Low-Energy Truly Random Number Generation with Superparamagnetic Tunnel Junctions for Unconventional Computing
Source: arXiv:1706.05262 ancillary file (2017-11-24)
Supplement: Supplementary file 1 [file supplementary.pdf]

# Low-Energy Truly Random Number Generation with Superparamagnetic Tunnel Junctions for Unconventional Computing
# (SUPPLEMENTARY MATERIAL)

D. Vodenicarevic,[1] N. Locatelli,[1] A. Mizrahi,[1,2] J. S. Friedman,[3] A. F. Vincent,[1] M. Romera,[2] A. Fukushima,[4] K. Yakushiji,[4] H. Kubota,[4] S. Yuasa,[4] S. Tiwari,[5] J. Grollier,[2] and D. Querlioz[1]

[1]*Centre for Nanoscience and Nanotechnology, CNRS, Univ. Paris-Sud, Université Paris-Saclay, C2N Orsay, 91405 Orsay, France*
[2]*Unité Mixte de Physique CNRS, Thales, Univ. Paris-Sud, Université Paris-Saclay, 91767 Palaiseau, France*
[3]*University of Texas at Dallas, 800 West Campbell Road Richardson, TX 75080, USA*
[4]*AIST Tsukuba, 1-1-1 Higashi, Tsukuba, Ibaraki 305-8561, Japan*
[5]*School of ECE, Cornell University, Ithaca, New York 14850, USA*

(Dated: November 24, 2017)

## S1 - EFFECT OF WHITENING ON RANDOM BITSTREAM QUALITY

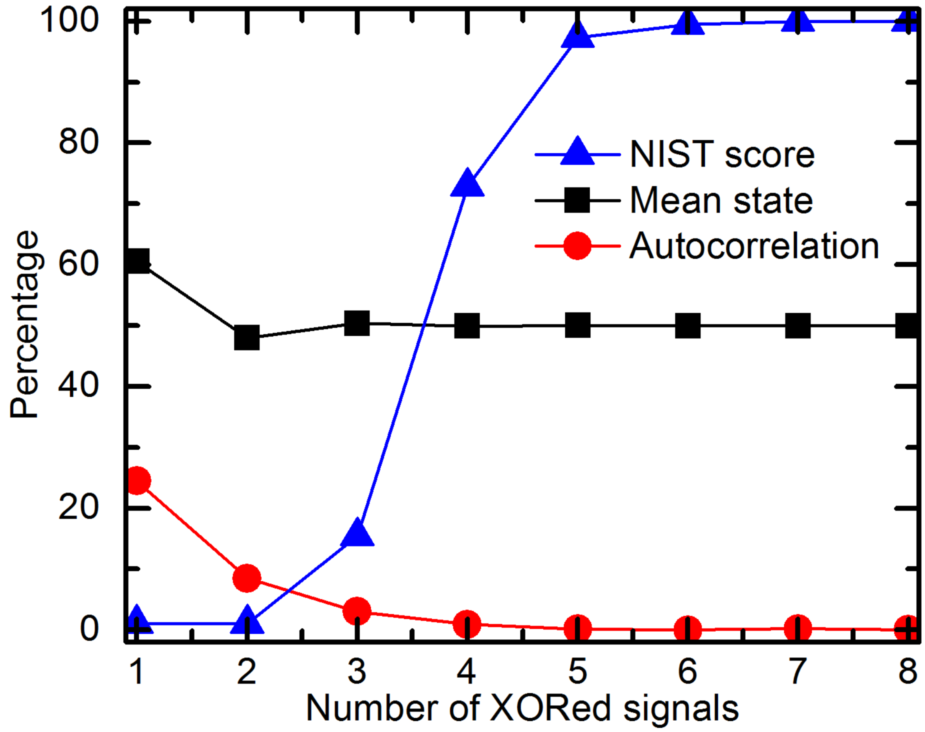


Figure 1. **Effect of whitening on random bitstream quality.** NIST STS score, mean state and consecutive bit correlation, obtained from the experimental random bitstream from subsampled at a rate of 5kHz, as functions of the number of XOR-combined signals.

## S2 - NIST STS RESULTS ON A SECOND JUNCTION

| $F_{\text{sampling}}$ | $F_{\text{sampling}}/F_{\text{MTJ}}$ | **Raw** | **XOR2** | **XOR4** | **XOR8** |
|---|---|---|---|---|---|
| 100 kHz | 71.4 | 0 | 10.1 | 10.1 | 10.1 |
| 20 kHz | 14.3 | 0.5 | 10.1 | 10.6 | 12.2 |
| 9.1 kHz | 6.5 | 10.6 | 10.6 | 12.8 | 89.9 |
| 5.9 kHz | 4.2 | 10.6 | 10.6 | 20.2 | 100 |
| 5 kHz | 3.6 | 10.6 | 10.6 | 84.6 | 100 |
| 1.9 kHz | 1.3 | 14.9 | 90.4 | 100 | 100 |
| 0.9 kHz | 0.6 | 13.3 | 97.9 | 100 | 100 |
| 0.7 kHz | 0.5 | 8.5 | 95.7 | 99.5 | 100 |
| 0.5 kHz | 0.4 | 11.7 | 96.3 | 100 | 100 |

Table I. **NIST STS results on a second junction.** Percentage of NIST STS tests satisfying cryptographic quality requirements, based on measurements on a second junction, for different numbers of combined bit-streams, and different sampling frequencies. The junction was measured under a $0.45\text{mT}$ external magnetic field. The mean switching frequency of the junction was measured to be $F_{\text{MTJ}} = 1.40\text{kHz}$.

---

## S3 - DISCUSSION ON SUPERPARAMAGNETIC JUNCTION SWITCHING PROCESS

In the case of our $50 \times 150\text{nm}$ superparamagnetic tunnel junctions, our results suggest that device switching occurs through nucleation and propagation of a magnetic domain, probably seeded by fluctuations in a subset of grains within it (by opposition to single domain magnetic reversal). The small effective switching volume of the free ferromagnet involved in the nucleation of the switching process explains the low energy barriers observed between the stable states, as compared to the full volume reversal energy barrier expected for those dimensions (evaluated to be approximately 126kT).

## S4 - SAMPLING FREQUENCY AND CORRELATION BETWEEN CONSECUTIVE SAMPLES

The auto-correlation function of a telegraphic signal can be derived simply from its escape rates, allowing to express the average correlation between consecutive samples as :

$$\rho_{X,X+1}(T_{sampling}) = e^{-(r_{0\to1}+r_{1\to0})\,T_{sampling}} \quad (1)$$

where $r_{0\to1}$ and $r_{1\to0}$ are the escape rates from $0$ and $1$ states respectively, and $T_{sampling}$ is the sampling period.
In case of a symmetrical system with $r_{0\to1} = r_{1\to0} = f_0 \exp\left(-\frac{\Delta E}{k_B T}\right) = 2F_{\mathrm{MTJ}}$, the maximal sampling frequency is then obtained knowing the critical correlation $\rho^c_{X,X+1}$ that can be mitigated by the whitening operation :

$$F^{\mathrm{max}}_{\mathrm{sampling}} = \frac{4F_{\mathrm{MTJ}}}{\ln(1/\rho^c_{X,X+1})} = \frac{2f_0}{\ln(1/\rho^c_{X,X+1})} \exp\left(-\frac{\Delta E}{k_B T}\right) \quad (2)$$

$F^{max}_{sampling} = 3F_{MTJ} = \frac{3}{2} f_0 \exp\left(-\frac{\Delta E}{k_B T}\right)$ corresponds to a critical correlation $\rho^c_{X,X+1} \approx 26\%$.

## S5 - CROSSTALK THROUGH DIPOLAR INTERACTION

We model the free magnetic layers of two identical side by side superparamagnetic tunnel junctions as two dipoles that interacts by dipolar interactions (Fig. 2(a)).

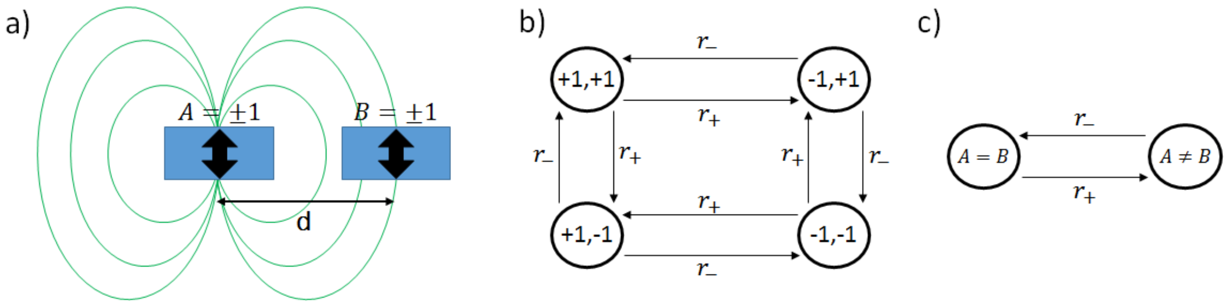


Figure 2. **Crosstalk through dipolar interaction.** **(a)** Representation of the free magnetic layers of two identical side by side superparamagnetic tunnel junctions modeled as two dipoles. Their state is associated respectively to the variables $A$ and $B$ taking two possible values $\{+1, -1\}$. **(b)** 4-states Markov chain showing the possible transitions between all {A,B} system states, and associated transition rates. **(c)** Simplified Markov chain.

The two superparamagnetic tunnel junctions constitute a stochastic system described as a 4-states markov process[1] (Fig. 2(b)). Their states are models by two variables $\{A, B\}$ that can take two values $\{-1, +1\}$. In the absence of interaction, the transition rates would be strictly identical, $r = f_0 \exp\left(-\frac{\Delta E}{k_B T}\right)$, but dipolar interaction will create an asymmetry so that two different rates have to be considered[2]:

$$\begin{cases} r_+ = f_0 \exp\left(-\dfrac{\Delta E}{k_B T}\left(1 + \dfrac{H_{dip}}{H_k}\right)^2\right) \\ r_- = f_0 \exp\left(-\dfrac{\Delta E}{k_B T}\left(1 - \dfrac{H_{dip}}{H_k}\right)^2\right) \end{cases} \tag{3}$$

where $H_k = \frac{2\Delta E}{k_B T}$ is the magnetic layer's coercive field and $H_{dip}$ is the amplitude of the dipolar field radiated by one junction on the other given by : $H_{dip} = \frac{M_S V}{4\pi d^3}$
This system can be simplified as a 2 states system (Fig. 2(c)):

$$\begin{cases} \partial_t P_{A=B} = +r_- P_{A\neq B} - r_+ P_{A=B} \\ \partial_t P_{A\neq B} = -r_- P_{A\neq B} + r_+ P_{A=B} \end{cases} \tag{4}$$

with stationary solutions : $P_{A=B} = \frac{r_+}{r_+ + r_-}$ and $P_{A\neq B} = \frac{r_-}{r_+ + r_-}$.
The cross-correlation between the two junctions state is then expressed as :

$$\rho = \frac{|\langle AB \rangle|}{\sqrt{\langle A^2 \rangle \langle B^2 \rangle}} = |\langle AB \rangle| = P_{A\neq B} - P_{A=B} \tag{5}$$

Using expressions from system (3), we then obtain :

$$\rho = \tanh\left(2\frac{\Delta E}{k_B T}\frac{H_{dip}}{H_k}\right) \tag{6}$$

Replacing expressions of dipolar and coercive fields:

$$\rho = \tanh\left(\frac{\mu_0 (M_S V)^2}{4\pi k_B T d^3}\right) \tag{7}$$

Given a target critical cross-correlation, we finally obtain the critical interdistance between two superparamagnetic tunnel junctions:

$$d_c = \left(\frac{\mu_0 (M_S V)^2}{4\pi k_B T \tanh^{-1}(\rho_c)}\right)^{1/3} \tag{8}$$

---

### S6 - SPAM DETECTOR: EMAIL CLASSIFIER ARCHITECTURE

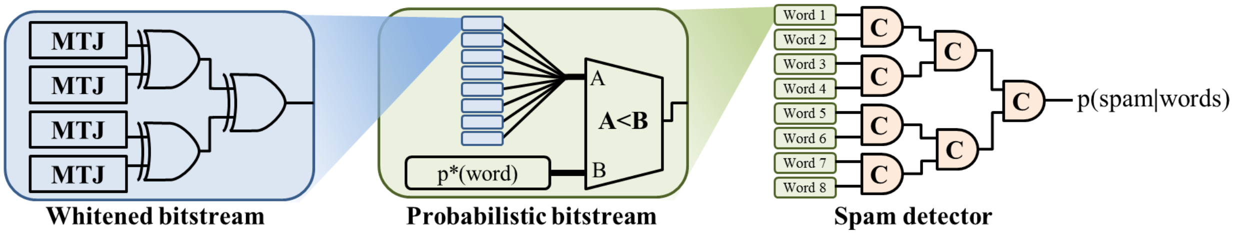


Figure 3. **Email classifier architecture.** Multi-scale schematic of the spam detector showing the whitened random bitstream generators (blue), the probabilistic bitstream generators using comparators (green) and the global C-Element inference circuit.

## S7 - EFFECT OF WHITENING ON SPAM DETECTION

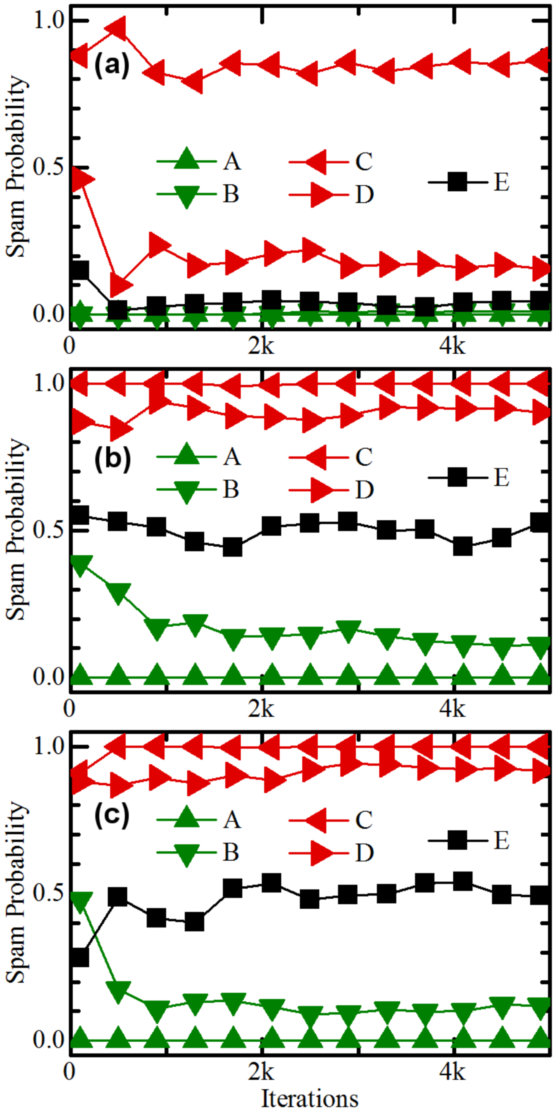


Figure 4. **Effect of whitening on spam detection.** Spam probabilities obtained using eight experimental random bits per word for the different sentences, as a function of the number of averaging iterations **(a)** without whitening, **(b)** with XOR4 whitening, **(c)** with XOR8 whitening

## S8 - EFFECT OF THE NUMBER OF BITS PER WORD ON SPAM DETECTION

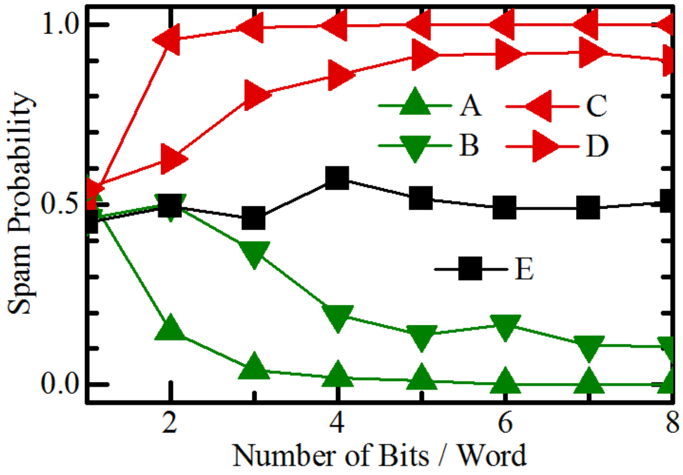


Figure 5. **Effect of the number of bits per word on spam detection.** Spam probabilities obtained using experimental random bits with 2,000-iteration averaging for the different sentences, as a function of the random number bit depth.

---

## S9 - ENERGY CONSUMPTION OF SPAM DETECTION

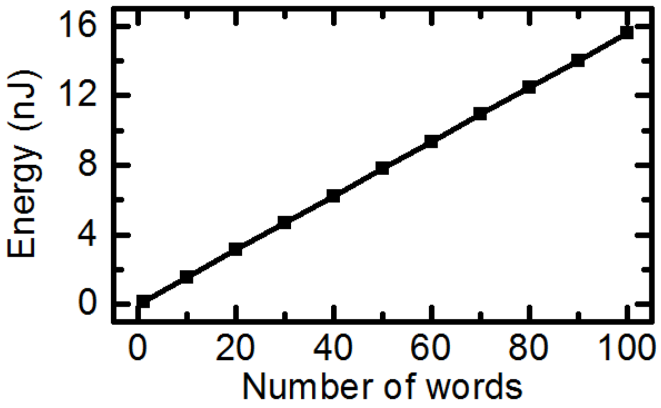


Figure 6. **Energy consumption of spam detection.** Total energy required to classify e-mail messages, as a function of the number of words in the dictionary.

## S10 - EFFECTS OF XOR WHITENING ON BITSTREAM PROBABILITY AND AUTO-CORRELATION

Our results show that applying XOR whitening allows to pass all the NIST tests at higher sampling rates (see tables in article and S2). This is due to XOR combining the randomness of independent, individually lower quality bitstreams into a high quality one, with lower auto-correlation, and a mean value closer to 0.5.

Here we demonstrate mathematically that a XOR gate combines two independent bitstreams $A$ and $B$ into a whitened bitstream $S = \mathrm{XOR}(A, B)$ that has lower auto-correlation and a mean value closer to 0.5 than both $A$ and $B$. We assume $P(A) \in (0;1)$ and $P(B) \in (0;1)$.

### Auto-correlation

Auto-correlation can arise in consecutive samples of the bitstreams at $t_1$ and $t_2 = t_1 + \mathrm{dt}$. We define $A_1$ and $A_2$ as the two samples of $A$ at $t_1$ and $t_2$ respectively. The same goes with $B_1$ and $B_2$ for bitstream $B$, and $S_1, S_2$ for the output bitstream $S$. We assume that all the probabilities are stable in time (for example $P(A_1) = P(A_2) = P(A)$). The conditional probability $P(A_1|A_2)$ can be reversed using the Bayes theorem, and shows the following symmetry:

$$P(A_1|A_2) = \frac{P(A_1)}{P(A_2)} P(A_2|A_1) = P(A_2|A_1) \tag{9}$$

Which also applies to $P(B_1|B_2)$ and $P(S_1|S_2)$.
We also have:

$$\begin{aligned} P(A_2 \cap \bar{A}_1) &= (1 - P(A))P(A_2|\bar{A}_1) = (1 - P(A))\frac{P(A)}{1 - P(A)} P(\bar{A}_1|A_2) \\ &= P(A)\big(1 - P(A_2|A_1)\big) \end{aligned} \tag{10}$$

and

$$P(\bar{A}_2 \cap A_1) = P(A)P(\bar{A}_2|A_1) = P(A)\big(1 - P(A_2|A_1)\big) \tag{11}$$

This implies the symmetry $P(\bar{A}_2 \cap A_1) = P(A_2 \cap \bar{A}_1)$.
We define the probability of the two samples $A_1$ and $A_2$ being equal as:

$$P(A_2 = A_1) = P\left((A_2 \cap A_1) \cup \left(\bar{A}_2 \cap \bar{A}_1\right)\right) = P\left(A_2 \cap A_1\right) + P\left(\bar{A}_2 \cap \bar{A}_1\right) \tag{12}$$

Moreover, the sum of the probabilities of all the outcomes on $A_1$ and $A_2$ is one:

$$P(\bar{A}_2 \cap \bar{A}_1) + P(A_2 \cap A_1) + P(\bar{A}_2 \cap A_1) + P(A_2 \cap \bar{A}_1) = 1 \tag{13}$$

By identifying $P(A_2 = A_1)$ and using the symmetry $P(\bar{A}_2 \cap A_1) = P(A_2 \cap \bar{A}_1)$ in this equation we get:

$$P(\bar{A}_2 \cap A_1) = P(A_2 \cap \bar{A}_1) = \frac{1 - P(A_2 = A_1)}{2} \tag{14}$$

Note that these results also apply to $B$ and $S$.
The output of the XOR gate is equal for the two consecutive samples ($S_2 = S_1$) in the following cases:

- $A_1 = 0, B_1 = 0, A_2 = 0, B_2 = 0$ ; with probability $P(\bar{A}_2 \cap \bar{A}_1)P(\bar{B}_2 \cap \bar{B}_1)$
- $A_1 = 0, B_1 = 0, A_2 = 1, B_2 = 1$ ; with probability $P(A_2 \cap \bar{A}_1)P(B_2 \cap \bar{B}_1)$
- $A_1 = 1, B_1 = 1, A_2 = 0, B_2 = 0$ ; with probability $P(\bar{A}_2 \cap A_1)P(\bar{B}_2 \cap B_1)$
- $A_1 = 1, B_1 = 1, A_2 = 1, B_2 = 1$ ; with probability $P(A_2 \cap A_1)P(B_2 \cap B_1)$
- $A_1 = 0, B_1 = 1, A_2 = 0, B_2 = 1$ ; with probability $P(\bar{A}_2 \cap \bar{A}_1)P(B_2 \cap B_1)$
- $A_1 = 0, B_1 = 1, A_2 = 1, B_2 = 0$ ; with probability $P(A_2 \cap \bar{A}_1)P(\bar{B}_2 \cap B_1)$
- $A_1 = 1, B_1 = 0, A_2 = 0, B_2 = 1$ ; with probability $P(\bar{A}_2 \cap A_1)P(B_2 \cap \bar{B}_1)$
- $A_1 = 1, B_1 = 0, A_2 = 1, B_2 = 0$ ; with probability $P(A_2 \cap A_1)P(\bar{B}_2 \cap \bar{B}_1)$

The probability $P(S_2 = S_1)$ is obtained by summing those probabilities. After summing, factoring and using the $P(\bar{A}_2 \cap A_1) = P(A_2 \cap \bar{A}_1)$ symmetry we get:

$$\begin{aligned} P(S_2 = S_1) =& 4P(A_2 \cap \bar{A}_1)P(B_2 \cap \bar{B}_1) \\ &+ \big(P(A_2 \cap A_1) + P(\bar{A}_2 \cap \bar{A}_1)\big)\big(P(B_2 \cap B_1) + P(\bar{B}_2 \cap \bar{B}_1)\big) \end{aligned} \tag{15}$$

By identifying $P(A_2 = A_1)$ and $P(B_2 = B_1)$ we obtain the formula:

$$P(S_2 = S_1) = 1 - P(A_2 = A_1) - P(B_2 = B_1) + 2P(A_2 = A_1)P(B_2 = B_1) \tag{16}$$

from which the auto-correlation $\rho^S_{t_1,t_2}$ of the output bitstream $S$ is deduced using $\rho^S_{t_1,t_2} = P(S_2 = S_1) - P(S_2 \neq S_1)$, and similar expressions for $A$ and $B$ (called $\rho^A_{t_1,t_2}$ and $\rho^B_{t_1,t_2}$):

$$\begin{aligned} \rho^S_{t_1,t_2} &= P(S_2 = S_1) - P(S_2 \neq S_1) = 2P(S_2 = S_1) - 1 \\ &= 1 - 2P(A_2 = A_1) - 2P(B_2 = B_1) + 4P(A_2 = A_1)P(B_2 = B_1) \\ &= \rho^A_{t_1,t_2} \times \rho^B_{t_1,t_2} \end{aligned} \tag{17}$$

This result shows that the auto-correlation of the XOR output is always lower in magnitude than the auto-correlation of any of its inputs.

Moreover, the output of a XOR gate can be safely used as an input of another one for further whitening. Since the XOR operation is associative, XOR whitening can both be organized as a tree or a chain. The auto-correlation obtained after whitening $N$ independent MTJ signals $\{A_1, A_2, \cdots, A_N\}$ is therefore the product of all the individual auto-correlations of the MTJ signals:

$$\rho^S_{t_1,t_2} = \prod_{i=1}^{N} \rho^{A_i}_{t_1,t_2} \tag{18}$$

As a result, the magnitude of the auto-correlation after XOR whitening decreases exponentially on average with the number of combined MTJ signals. Highly correlated MTJ signals still contribute to this reduction, but less than the ones with low auto-correlation.

**Mean value**

The mean value $P(S)$ after XOR(A,B) is :

$$\begin{aligned} P(S) &= P\big((A \cap \bar{B}) \cup (\bar{A} \cap B)\big) = P(A)\big(1 - P(B)\big) + \big(1 - P(A)\big)P(B) \\ &= P(A) + P(B) - 2P(A)P(B) \end{aligned} \tag{19}$$

The normalized difference between the ideal $0.5$ mean value and $P(S)$ is $P(\bar{S}) - P(S) = 2\big(0.5 - P(S)\big)$. The same is defined for input $A$ with $2\big(0.5 - P(A)\big)$ and input B with $2\big(0.5 - P(B)\big)$. The previous expression of $P(S)$ can be rearranged to obtain:

$$2\big(0.5 - P(S)\big) = 2\big(0.5 - P(A)\big) \times 2\big(0.5 - P(B)\big) \tag{20}$$

When $P(A) = 0.5$ or $P(B) = 0.5$, we get $P(S) = 0.5$. Otherwise, we get the equivalence:

$$2\big|0.5 - P(S)\big| < 2\big|0.5 - P(A)\big| \Leftrightarrow 2\big|0.5 - P(B)\big| < 1 \tag{21}$$

which is always true.
These results show that the mean value at the output of a XOR gate is always closer to 0.5 than the mean value of any of its inputs, or equal to 0.5 if any of the inputs has already a mean value of exactly 0.5. In the case of $N$ combined signals $\{A_1, A_2, \cdots, A_N\}$, the mean value of the whitened signal follows:

$$2\big(0.5 - P(S)\big) = \prod_{i=1}^{N} 2\big(0.5 - P(A_i)\big) \tag{22}$$

This shows that the mean value of the whitened signal gets exponentially closer on average to $50\%$ as the number of combined signals increases. Again, better-balanced signals contribute more to balancing the whitened bitstream than highly unbalanced ones.

As a conclusion, this study shows that XOR whitening reduces auto-correlations exponentially with the number of combined signals and brings the mean value exponentially closer to $50\%$ with the number of combined signals.

**S11 - READ DISTURB EFFECT**

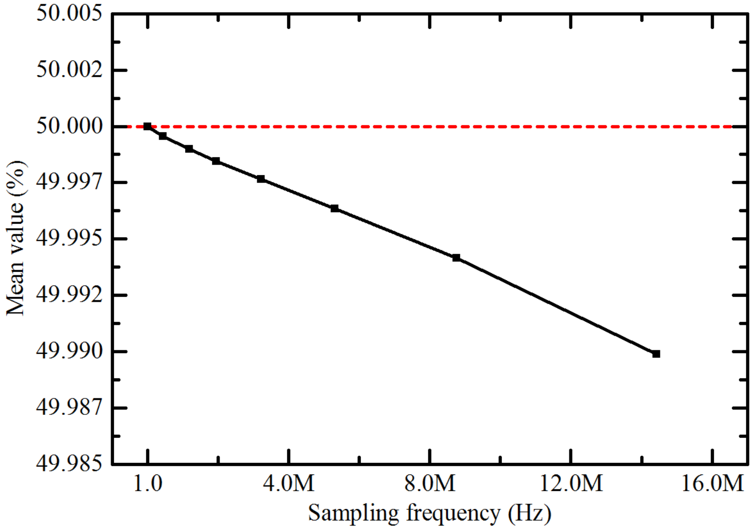


Figure 7. **Read disturb effect.** Mean value of a perfectly balanced ultrascaled stochastic MTJ as a function of the sampling frequency, obtained through SPICE simulation of the PCSA circuit and using our device model. The dashed red line represents the ideal $50\%$ mean value.

[1] A. Neiman, L. Schimansky-Geier, F. Moss, B. Shulgin, J. J. Collins, Synchronization of noisy systems by stochastic signals. *Physical Review E* **60**, 284292 (1999).
[2] W. Rippard, R. Heindl, M. Pufall, S. Russek, A. Kos, Thermal relaxation rates of magnetic nanoparticles in the presence of magnetic fields and spin-transfer effects. *Physical Review B* **84**, 064439 (2011).
